# Supplementary material for: PartImageNet: A Large, High-Quality Dataset of Parts
Source: arXiv:2112.00933 source file (2022-12-16)
Supplement: Supplementary file 1 [file 07_supplementary.tex]

% \newpage
\section{Supplementary Materials}

\subsection{PartImageNet Dataset (Few-shot learning version) Details}
 
As described in the Experiment Section, we construct a new version of PartImageNet for few-shot learning. Is is organized in an another way by splitting non-overlapping classes into training, validation and testing set. The new split especially designed for Few-shot Learning contains 109 classes in training set, 19 classes in validation set and 30 classes in testing set. The complete list of classes for the is shown below:

\noindent \textbf{Train Classes}: \\
\small{
n02102040, n02102973, n02101388, n02100583, n02096585, n02096177, n02089867, \\
n02109961, n02098105, n02097474, n02091831, n02112137, n02124075, n02443114, \\
n02128385, n02129604, n02133161, n02132136, n02441942, n02510455, n02403003, \\
n02415577, n02423022, n02408429, n02412080, n02397096, n02356798, n02114367, \\
n02130308, n02422699, n02437312, n02090379, n02444819, n02422106, n02481823, \\
n02480855, n02483362, n02492035, n02493793, n02486410, n02487347, n02486261, \\
n02489166, n02488702, n02484975, n02492660, n02071294, n01443537, n01440764, \\
n02607072, n02536864, n01855672, n02025239, n02033041, n02009912, n02002724, \\
n02006656, n01608432, n01828970, n02058221, n01744401, n01742172, n01749939, \\
n01755581, n01753488, n01735189, n01729322, n01740131, n01728572, n01739381, \\
n01756291, n01729977, n01687978, n01688243, n01694178, n01693334, n01695060, \\
n01692333, n01698640, n01665541, n01669191, n01641577, n01630670, n01632458, \\
n01664065, n01644900, n03770679 ,n03977966, n03417042, n02701002, n03100240, \\
n03670208, n04037443, n03444034, n04252225, n03769881, n04465501, n03445924, \\
n04065272, n04146614, n03792782, n04482393, n03791053, n03947888, n04612504, \\
n02690373, n02823428, n03937543, n03983396}

\noindent \textbf{Val Classes}: \\
\small{
n02099601, n02109525, n02125311, n02442845, n02134084, n02483708, n02490219, \\
n01484850, n02514041, n02009229, n01614925, n01748264, n01689811, n01685808, \\
n02814533, n02930766, n04509417, n04483307, n04557648}

\noindent \textbf{Test Classes}: \\ 
\small{
n02101006, n02092339, n02085782, n02120079, n02134418, n02417914, n02447366, \\
n02480495, n02494079, n02493509, n01491361, n01494475, n02655020, n01824575, \\
n02017213, n01843065, n01734418, n01728920, n01697457, n01667114, n01667778, \\
n01644373, n03594945, n04285008, n04487081, n03785016, n02835271, n04147183, \\
n04552348, n04591713}

\subsection{Implementation details of Semantic Segmentation}

We train the Deeplabv3+ \cite{chen2018encoder} and Semantic FPN \cite{ak2019panopticfpn} models using SGD optimizer with a learning rate of 0.01 and momentum of 0.9 for 40K iterations. The SegFormer \cite{xie2021segformer} models are trained using AdamW optimizer for 40K iterations following the default setting of an initial value of 0.00006 and then a “poly” LR schedule with factor 1.0. 

\subsection{Part Discovery}

Existing works on part discovery mainly focus on unsupervised \cite{collins2018deep} and self-supervised \cite{hung2019scops} co-part segmentation which aim at producing consistent part segments in a set of images with no strong supervision. Here we adopt one representative method DFF \cite{collins2018deep} to train it on our PartImageNet. Since unsupervised and self-supervised methods are able to produce consistent part segments and these segments usually do not correspond to the manually annotated object parts. We do not report the quantitative results by computing the part-level intersection-over-union (IoU). Instead, we just show qualitative results here. As can be observed, in certain cases, DFF \cite{collins2018deep} can already produce satisfying results such as the goat. It segments the goat into four semantic parts, though these parts do not correspond to our manually annotation precisely, it is still meaningful and useful for downstream tasks. 
% However, the limitations of such unsupervised or self-supervised methods are also very obvious. They need to set a pre-defined number of parts before running the algorithm which makes it can not handle real situations well. Besides, they are also not robust to the transformation of shape and texture, during these situations, they are of high possibility to produce meaningless results.

\subsection{Visualization Results of Part Discovery}

\begin{figure*}[hb]
    \centering
    \begin{subfigure}{0.24\linewidth}
        \centering
        \includegraphics[width=\linewidth,height=\linewidth]{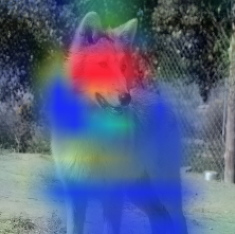}
    \end{subfigure}
    \begin{subfigure}{0.24\linewidth}
        \centering
        \includegraphics[width=\linewidth,height=\linewidth]{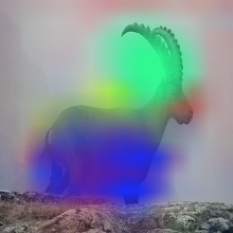}
    \end{subfigure}
    \begin{subfigure}{0.24\linewidth}
        \centering
        \includegraphics[width=\linewidth,height=\linewidth]{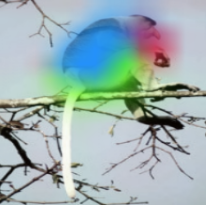}
    \end{subfigure}
    \begin{subfigure}{0.24\linewidth}
        \centering
        \includegraphics[width=\linewidth,height=\linewidth]{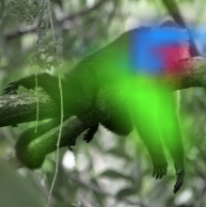}
    \end{subfigure}
    \begin{subfigure}{0.24\linewidth}
        \centering
        \includegraphics[width=\linewidth,height=\linewidth]{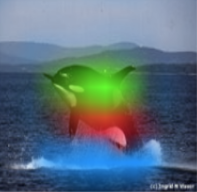}
    \end{subfigure}
    \begin{subfigure}{0.24\linewidth}
        \centering
        \includegraphics[width=\linewidth,height=\linewidth]{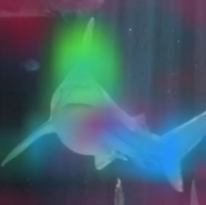}
    \end{subfigure}
    \begin{subfigure}{0.24\linewidth}
        \centering
        \includegraphics[width=\linewidth,height=\linewidth]{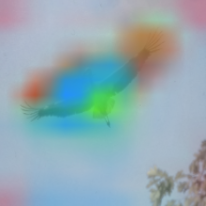}
    \end{subfigure}
    \begin{subfigure}{0.24\linewidth}
        \centering
        \includegraphics[width=\linewidth,height=\linewidth]{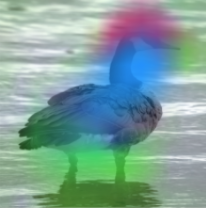}
    \end{subfigure}
    \begin{subfigure}{0.24\linewidth}
        \centering
        \includegraphics[width=\linewidth,height=\linewidth]{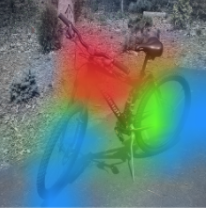}
    \end{subfigure}
    \begin{subfigure}{0.24\linewidth}
        \centering
        \includegraphics[width=\linewidth,height=\linewidth]{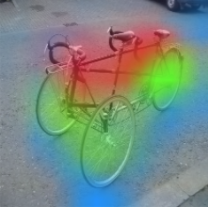}
    \end{subfigure}
    \begin{subfigure}{0.24\linewidth}
        \centering
        \includegraphics[width=\linewidth,height=\linewidth]{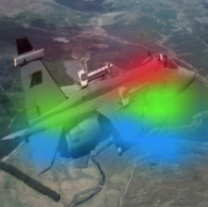}
    \end{subfigure}
    \begin{subfigure}{0.24\linewidth}
        \centering
        \includegraphics[width=\linewidth,height=\linewidth]{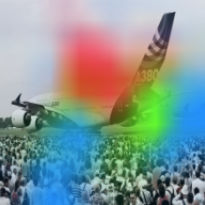}
    \end{subfigure}
    \caption{Visualization results of DFF \cite{collins2018deep} for Part Discovery.}
    \label{fig:discovery}
\end{figure*}

\subsection{Visualization of More Annotated Images}

\begin{figure*}[!h]
    \centering
    \begin{subfigure}{0.24\linewidth}
        \centering
        \includegraphics[width=\linewidth,height=\linewidth]{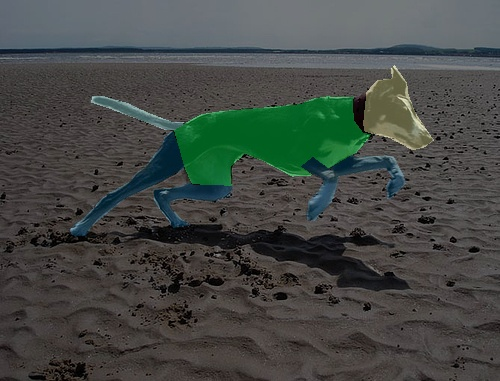}
    \end{subfigure}
    \begin{subfigure}{0.24\linewidth}
        \centering
        \includegraphics[width=\linewidth,height=\linewidth]{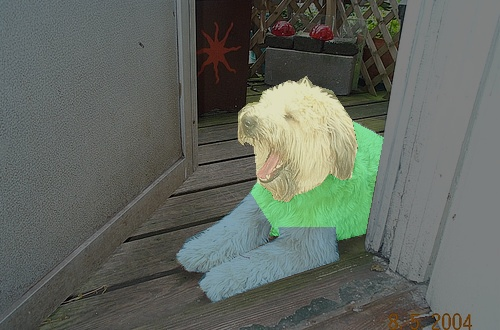}
    \end{subfigure}
    \begin{subfigure}{0.24\linewidth}
        \centering
        \includegraphics[width=\linewidth,height=\linewidth]{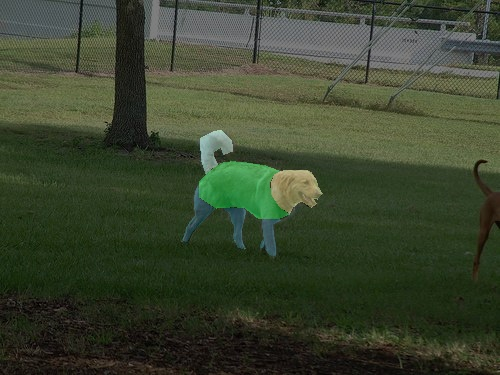}
    \end{subfigure}
    \begin{subfigure}{0.24\linewidth}
        \centering
        \includegraphics[width=\linewidth,height=\linewidth]{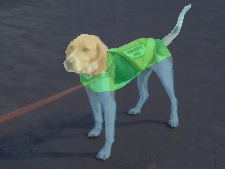}
    \end{subfigure}
    \begin{subfigure}{0.24\linewidth}
        \centering
        \includegraphics[width=\linewidth,height=\linewidth]{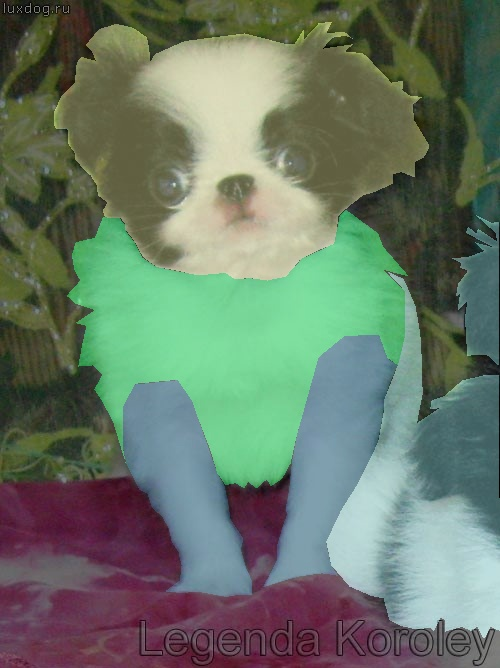}
    \end{subfigure}
    \begin{subfigure}{0.24\linewidth}
        \centering
        \includegraphics[width=\linewidth,height=\linewidth]{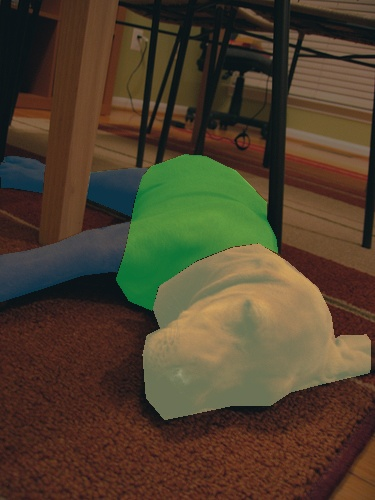}
    \end{subfigure}
    \begin{subfigure}{0.24\linewidth}
        \centering
        \includegraphics[width=\linewidth,height=\linewidth]{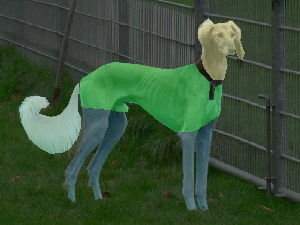}
    \end{subfigure}
    \begin{subfigure}{0.24\linewidth}
        \centering
        \includegraphics[width=\linewidth,height=\linewidth]{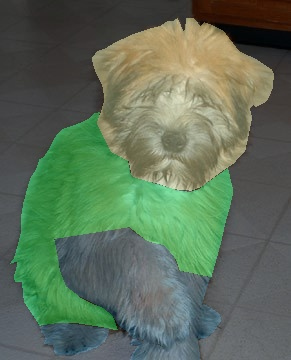}
    \end{subfigure}
    \begin{subfigure}{0.24\linewidth}
        \centering
        \includegraphics[width=\linewidth,height=\linewidth]{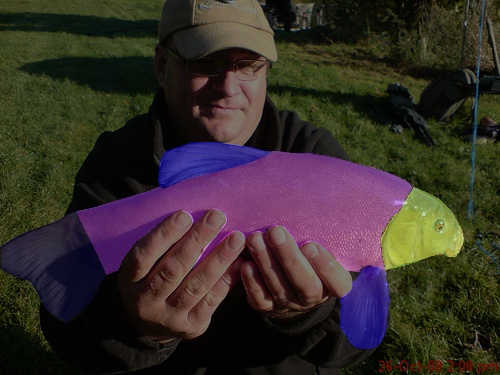}
    \end{subfigure}
    \begin{subfigure}{0.24\linewidth}
        \centering
        \includegraphics[width=\linewidth,height=\linewidth]{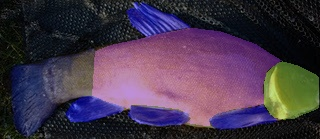}
    \end{subfigure}
    \begin{subfigure}{0.24\linewidth}
        \centering
        \includegraphics[width=\linewidth,height=\linewidth]{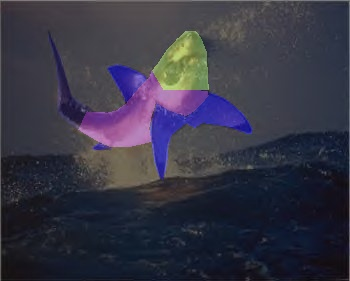}
    \end{subfigure}
    \begin{subfigure}{0.24\linewidth}
        \centering
        \includegraphics[width=\linewidth,height=\linewidth]{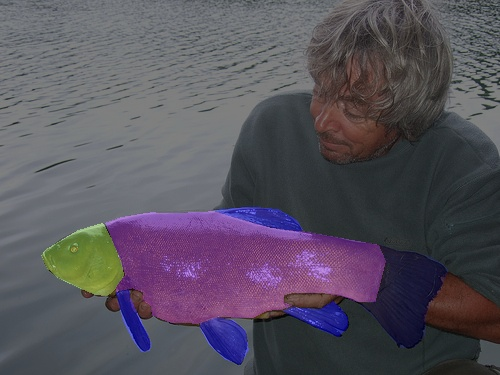}
    \end{subfigure}
    \begin{subfigure}{0.24\linewidth}
        \centering
        \includegraphics[width=\linewidth,height=\linewidth]{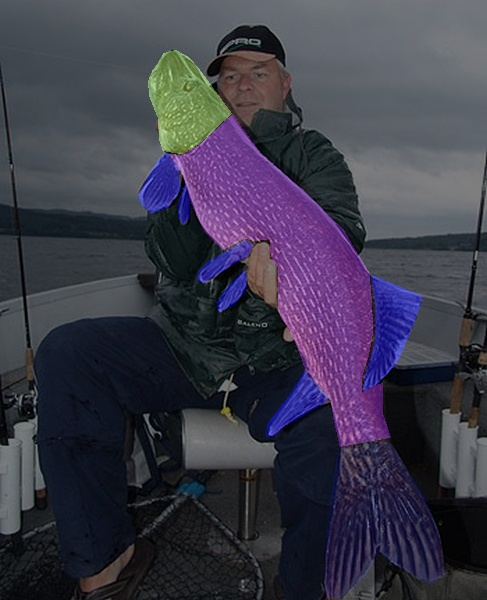}
    \end{subfigure}
    \begin{subfigure}{0.24\linewidth}
        \centering
        \includegraphics[width=\linewidth,height=\linewidth]{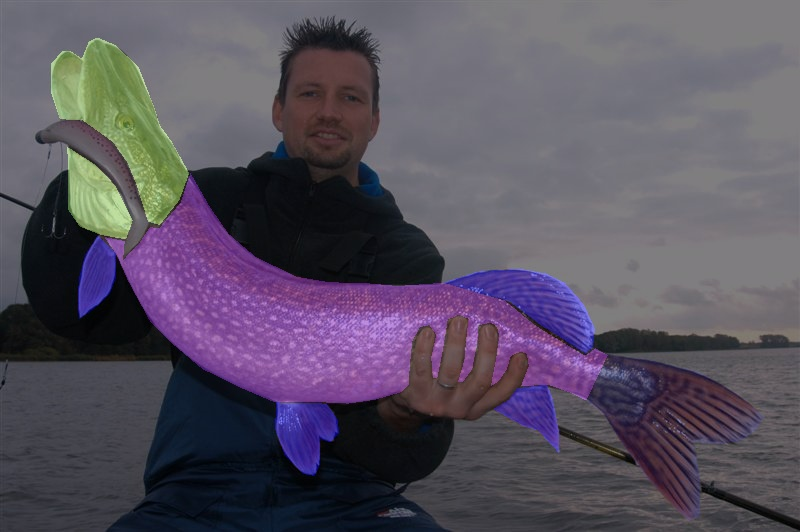}
    \end{subfigure}
    \begin{subfigure}{0.24\linewidth}
        \centering
        \includegraphics[width=\linewidth,height=\linewidth]{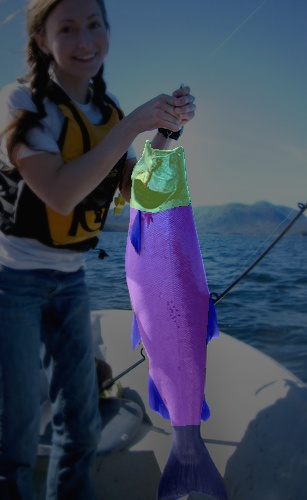}
    \end{subfigure}
    \begin{subfigure}{0.24\linewidth}
        \centering
        \includegraphics[width=\linewidth,height=\linewidth]{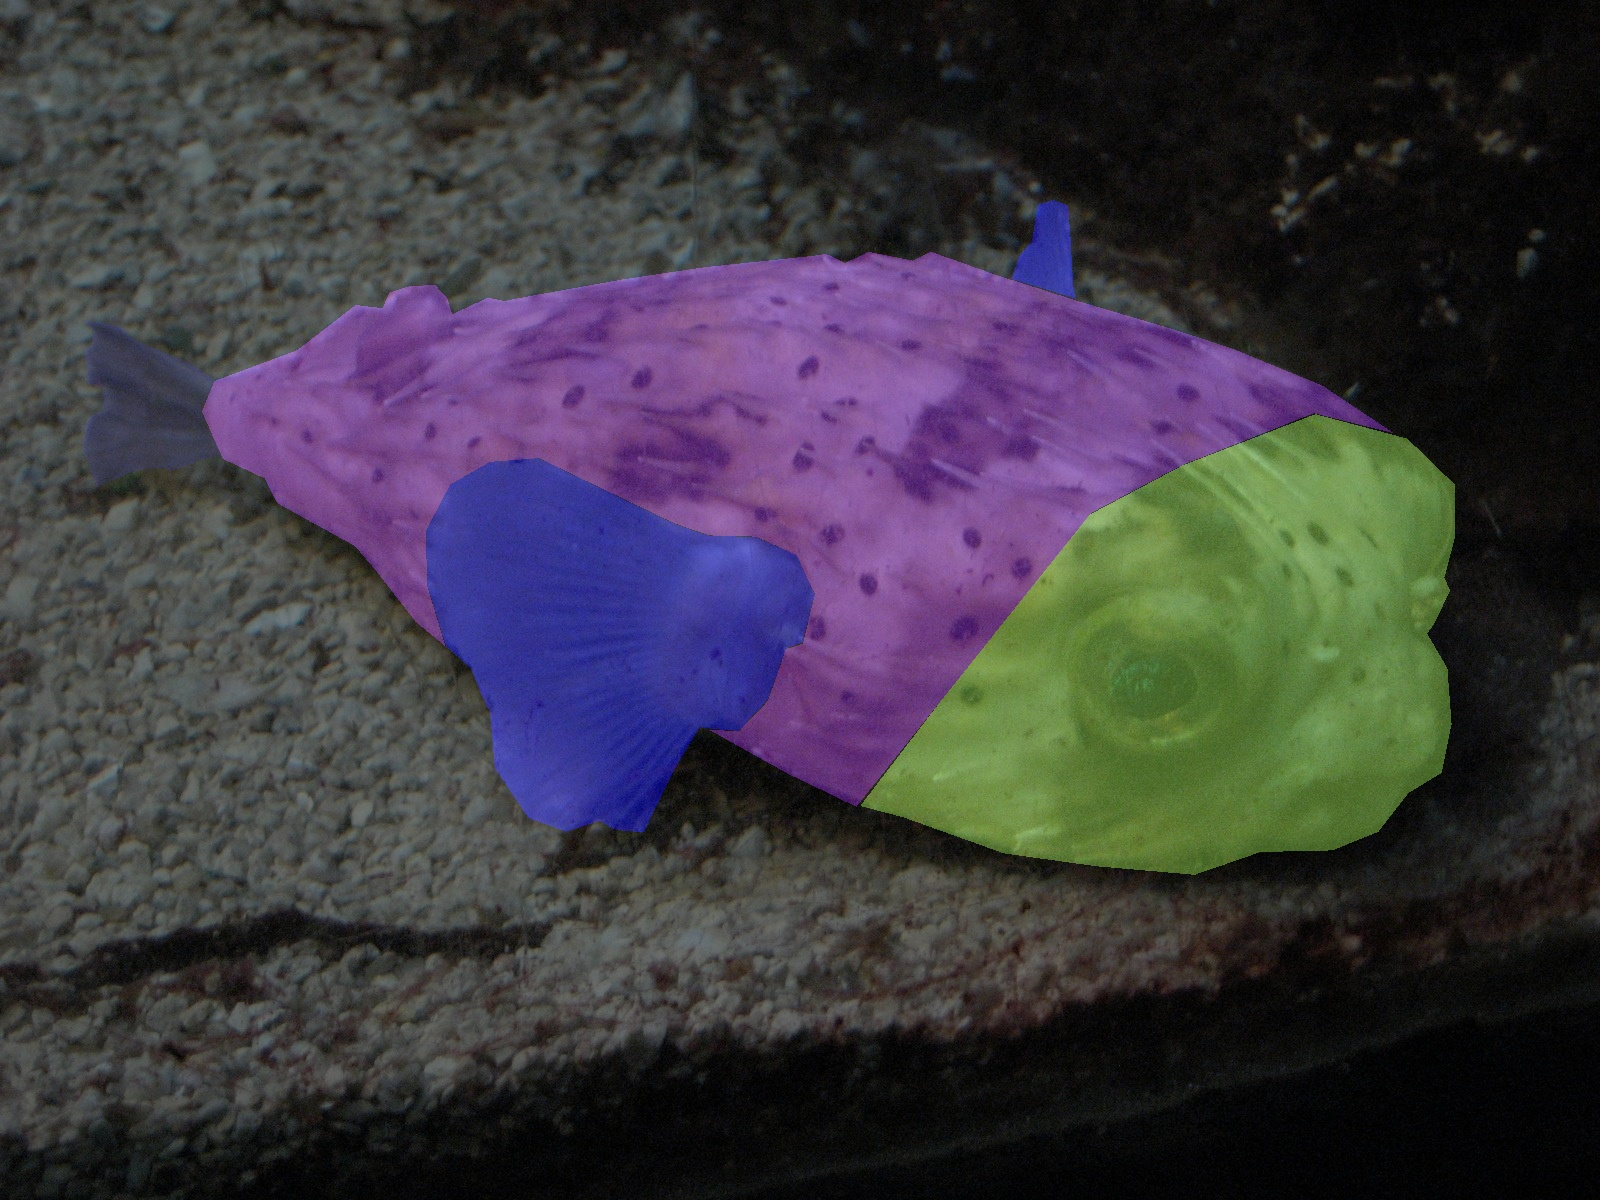}
    \end{subfigure}
    \begin{subfigure}{0.24\linewidth}
        \centering
        \includegraphics[width=\linewidth,height=\linewidth]{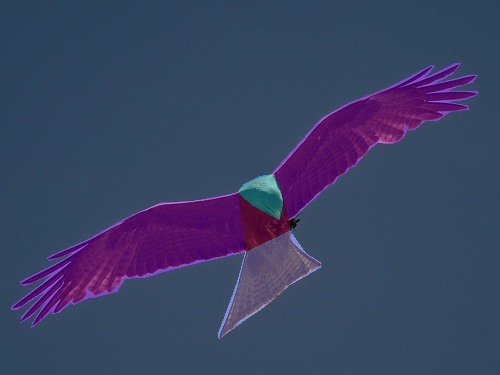}
    \end{subfigure}
    \begin{subfigure}{0.24\linewidth}
        \centering
        \includegraphics[width=\linewidth,height=\linewidth]{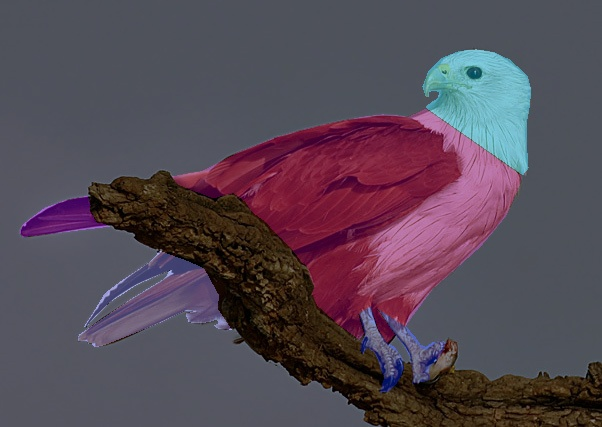}
    \end{subfigure}
    \begin{subfigure}{0.24\linewidth}
        \centering
        \includegraphics[width=\linewidth,height=\linewidth]{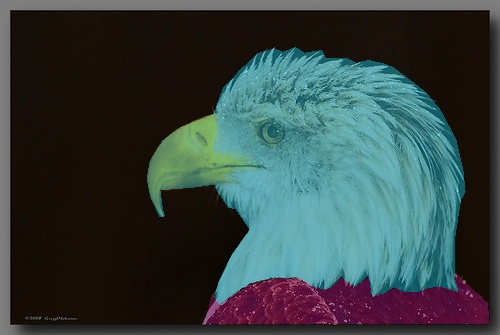}
    \end{subfigure}
    \begin{subfigure}{0.24\linewidth}
        \centering
        \includegraphics[width=\linewidth,height=\linewidth]{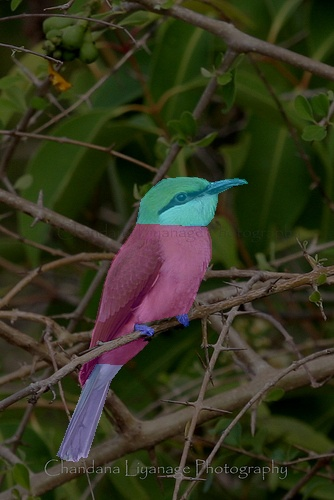}
    \end{subfigure}
    \begin{subfigure}{0.24\linewidth}
        \centering
        \includegraphics[width=\linewidth,height=\linewidth]{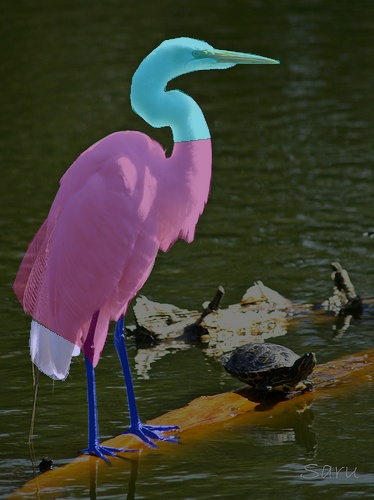}
    \end{subfigure}
    \begin{subfigure}{0.24\linewidth}
        \centering
        \includegraphics[width=\linewidth,height=\linewidth]{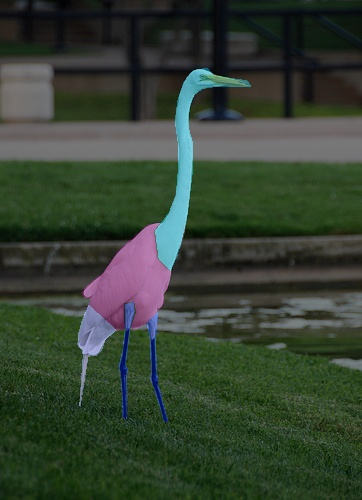}
    \end{subfigure}
    \begin{subfigure}{0.24\linewidth}
        \centering
        \includegraphics[width=\linewidth,height=\linewidth]{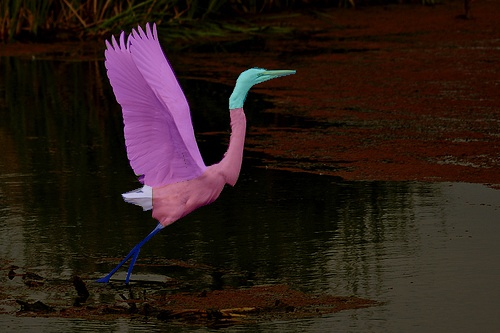}
    \end{subfigure}
    \begin{subfigure}{0.24\linewidth}
        \centering
        \includegraphics[width=\linewidth,height=\linewidth]{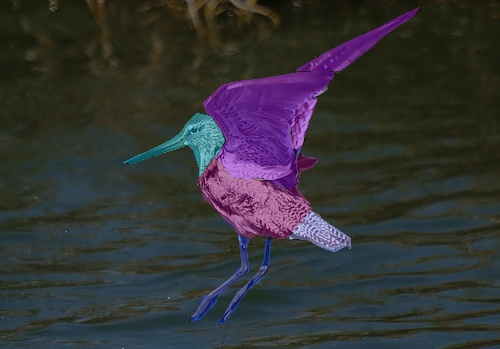}
    \end{subfigure}
\end{figure*}

\begin{figure*}
    \ContinuedFloat
    \centering
    \begin{subfigure}{0.24\linewidth}
        \centering
        \includegraphics[width=\linewidth,height=\linewidth]{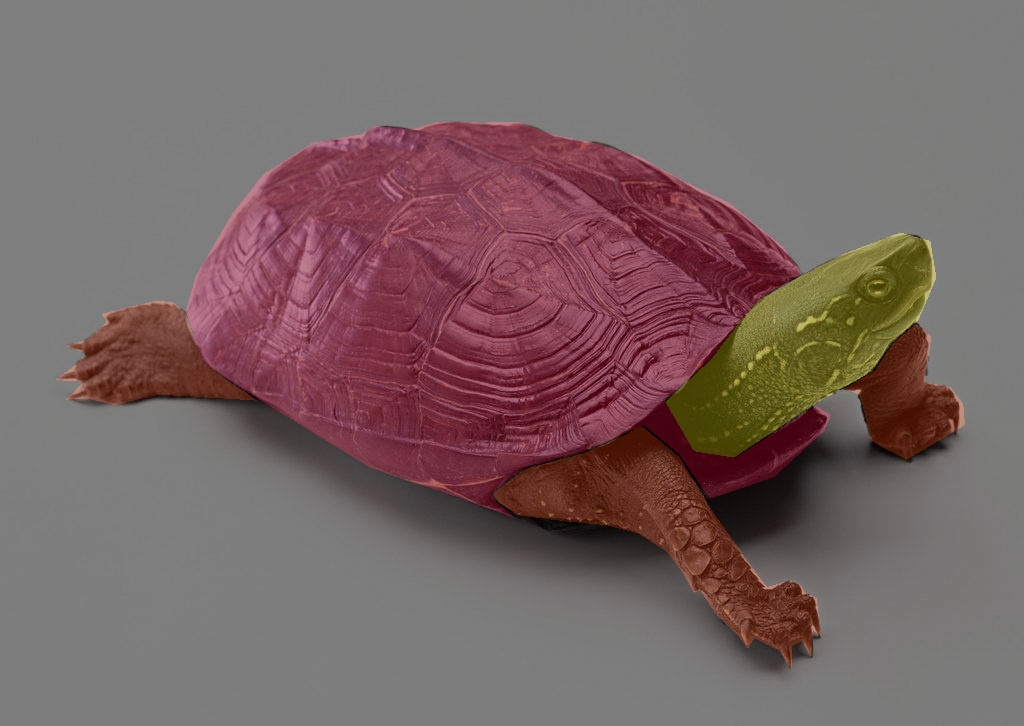}
    \end{subfigure}
    \begin{subfigure}{0.24\linewidth}
        \centering
        \includegraphics[width=\linewidth,height=\linewidth]{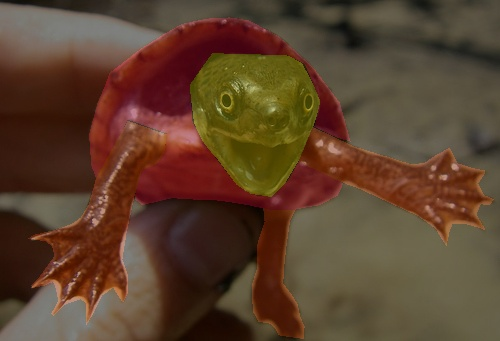}
    \end{subfigure}
    \begin{subfigure}{0.24\linewidth}
        \centering
        \includegraphics[width=\linewidth,height=\linewidth]{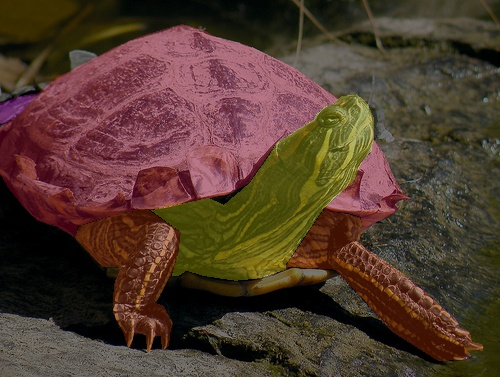}
    \end{subfigure}
    \begin{subfigure}{0.24\linewidth}
        \centering
        \includegraphics[width=\linewidth,height=\linewidth]{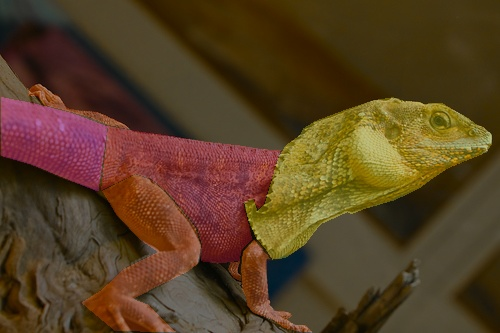}
    \end{subfigure}
    \begin{subfigure}{0.24\linewidth}
        \centering
        \includegraphics[width=\linewidth,height=\linewidth]{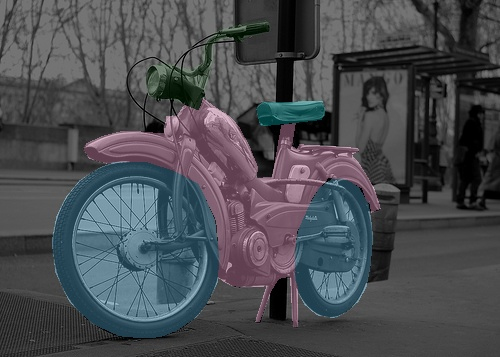}
    \end{subfigure}
    \begin{subfigure}{0.24\linewidth}
        \centering
        \includegraphics[width=\linewidth,height=\linewidth]{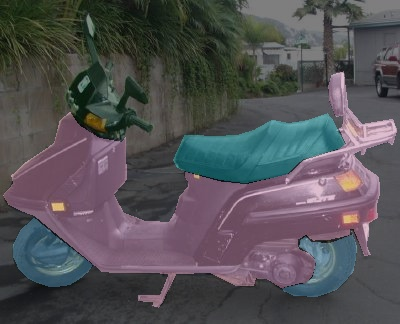}
    \end{subfigure}
    \begin{subfigure}{0.24\linewidth}
        \centering
        \includegraphics[width=\linewidth,height=\linewidth]{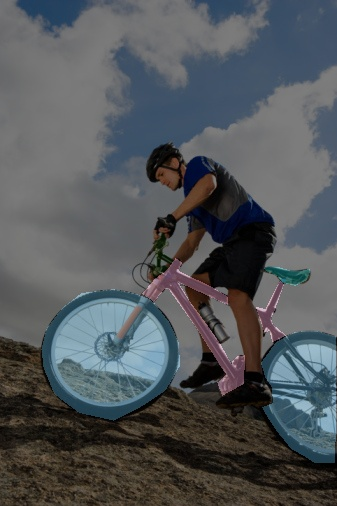}
    \end{subfigure}
    \begin{subfigure}{0.24\linewidth}
        \centering
        \includegraphics[width=\linewidth,height=\linewidth]{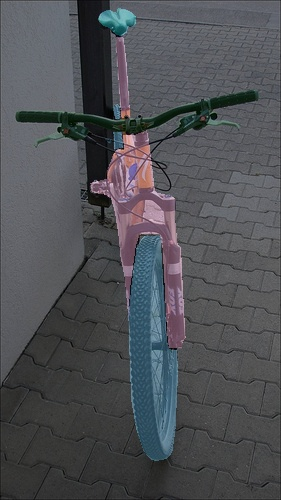}
    \end{subfigure}
    \begin{subfigure}{0.24\linewidth}
        \centering
        \includegraphics[width=\linewidth,height=\linewidth]{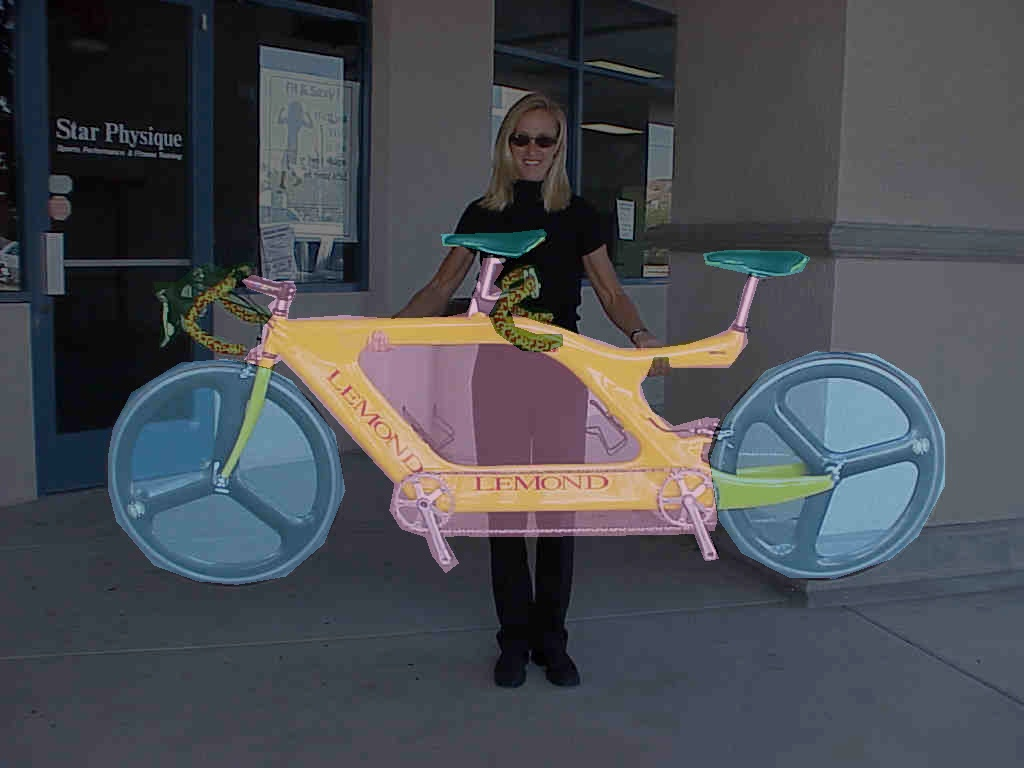}
    \end{subfigure}
    \begin{subfigure}{0.24\linewidth}
        \centering
        \includegraphics[width=\linewidth,height=\linewidth]{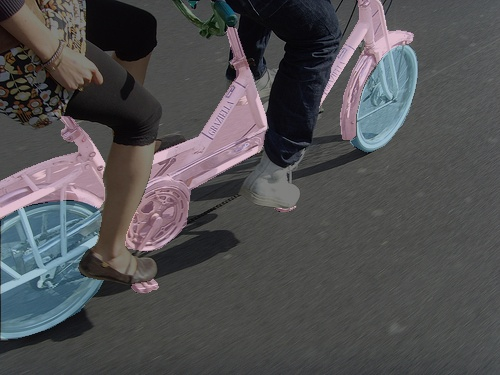}
    \end{subfigure}
    \begin{subfigure}{0.24\linewidth}
        \centering
        \includegraphics[width=\linewidth,height=\linewidth]{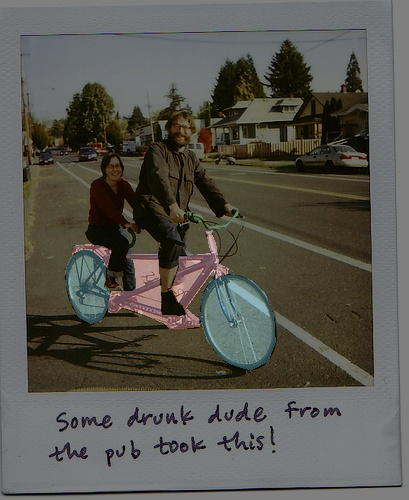}
    \end{subfigure}
    \begin{subfigure}{0.24\linewidth}
        \centering
        \includegraphics[width=\linewidth,height=\linewidth]{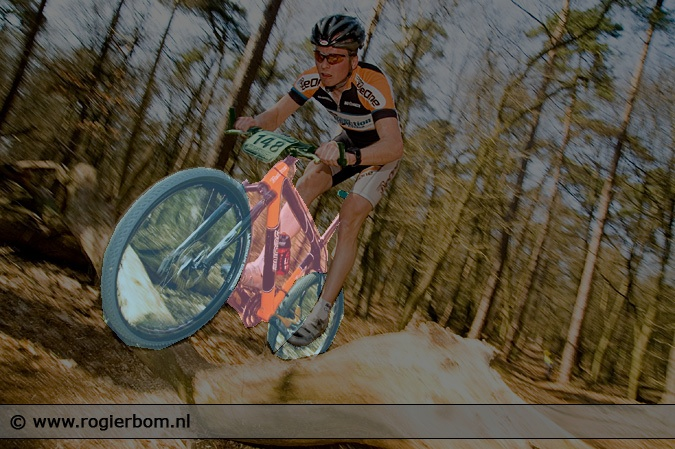}
    \end{subfigure}
    \begin{subfigure}{0.24\linewidth}
        \centering
        \includegraphics[width=\linewidth,height=\linewidth]{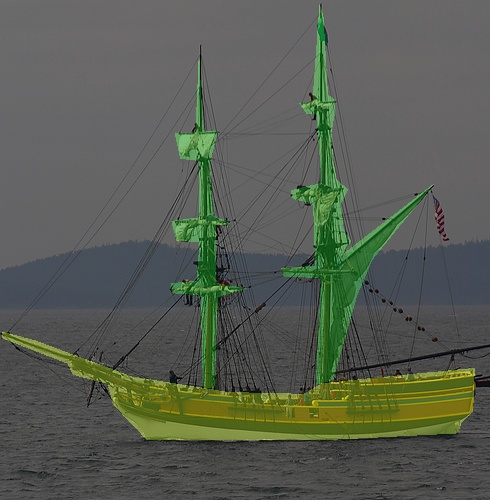}
    \end{subfigure}
    \begin{subfigure}{0.24\linewidth}
        \centering
        \includegraphics[width=\linewidth,height=\linewidth]{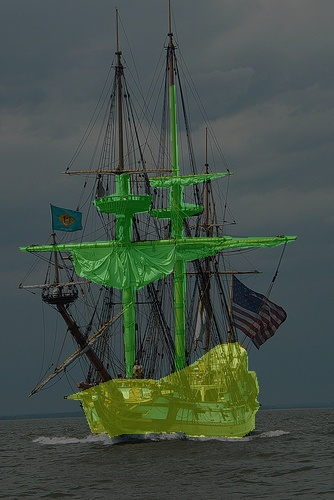}
    \end{subfigure}
    \begin{subfigure}{0.24\linewidth}
        \centering
        \includegraphics[width=\linewidth,height=\linewidth]{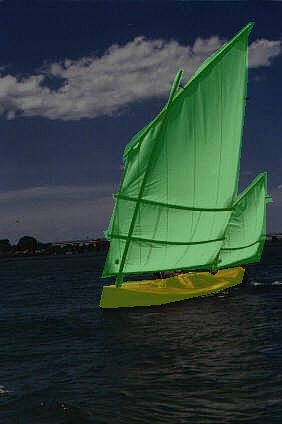}
    \end{subfigure}
    \begin{subfigure}{0.24\linewidth}
        \centering
        \includegraphics[width=\linewidth,height=\linewidth]{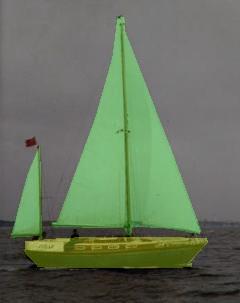}
    \end{subfigure}
    \begin{subfigure}{0.24\linewidth}
        \centering
        \includegraphics[width=\linewidth,height=\linewidth]{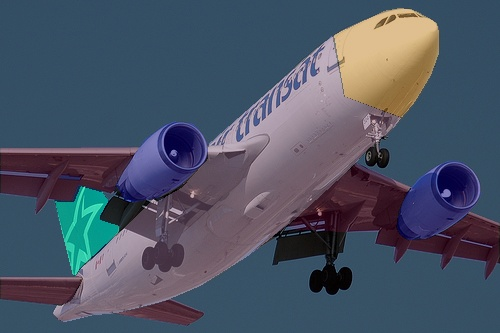}
    \end{subfigure}
    \begin{subfigure}{0.24\linewidth}
        \centering
        \includegraphics[width=\linewidth,height=\linewidth]{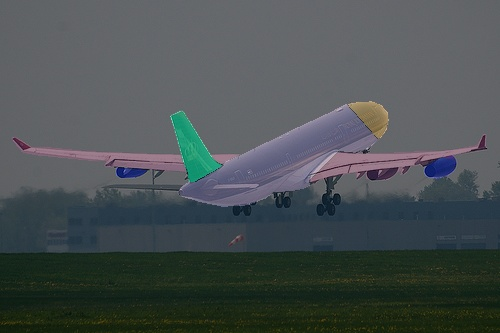}
    \end{subfigure}
    \begin{subfigure}{0.24\linewidth}
        \centering
        \includegraphics[width=\linewidth,height=\linewidth]{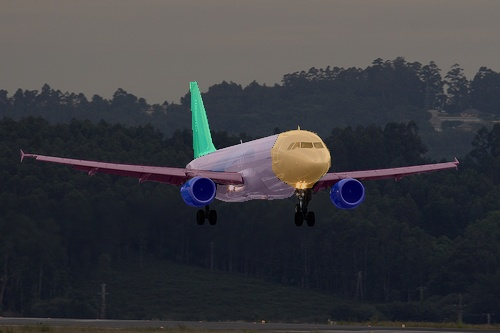}
    \end{subfigure}
    \begin{subfigure}{0.24\linewidth}
        \centering
        \includegraphics[width=\linewidth,height=\linewidth]{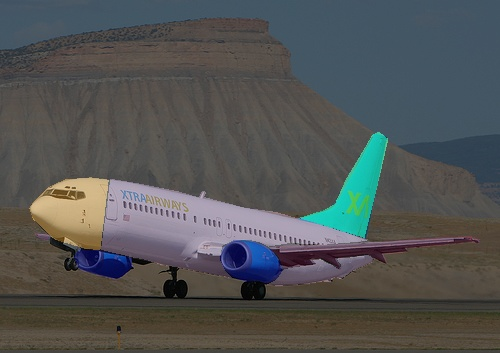}
    \end{subfigure}
    \begin{subfigure}{0.24\linewidth}
        \centering
        \includegraphics[width=\linewidth,height=\linewidth]{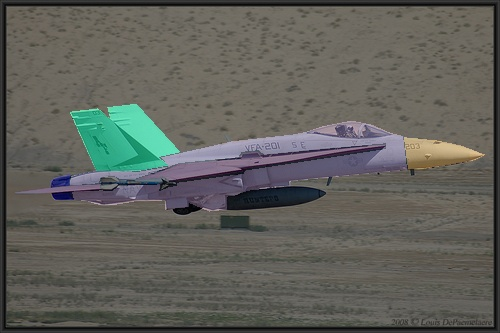}
    \end{subfigure}
    \begin{subfigure}{0.24\linewidth}
        \centering
        \includegraphics[width=\linewidth,height=\linewidth]{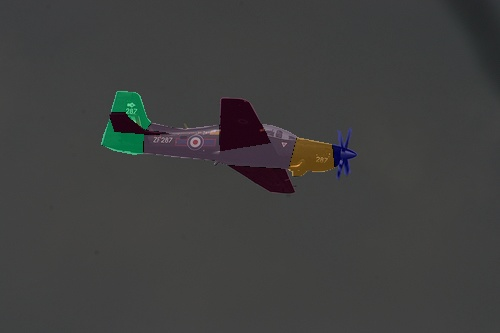}
    \end{subfigure}
    \begin{subfigure}{0.24\linewidth}
        \centering
        \includegraphics[width=\linewidth,height=\linewidth]{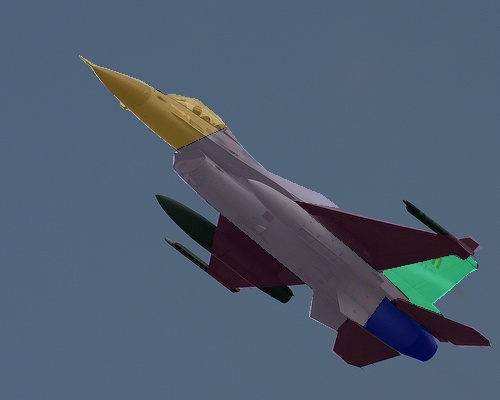}
    \end{subfigure}
    \begin{subfigure}{0.24\linewidth}
        \centering
        \includegraphics[width=\linewidth,height=\linewidth]{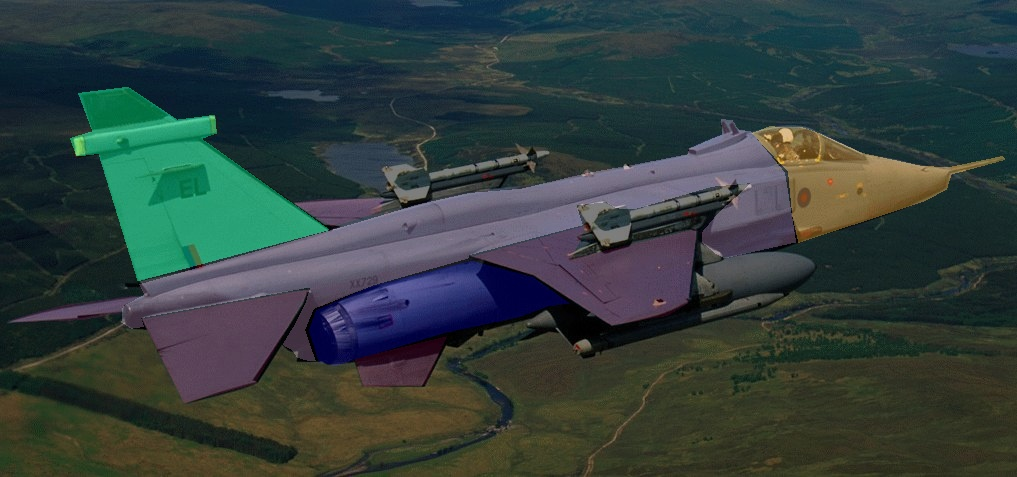}
    \end{subfigure}
    \caption{Visualization of more annotated images. We maintain a high-quality annotation with varying object classes, poses and background.}
    \label{fig:discovery}
\end{figure*}
